# Supplementary material for: AI-GOMS: Large AI-Driven Global Ocean Modeling System
Source: arXiv:2308.03152 source file (2023-08-10)
Supplement: Supplementary file 1 [file appendix.tex]

\begin{appendices}
\end{appendices}
